# Supplementary material for: Stringent limits on $C\!PT$- and Lorentz-invariance violation from $B_s^0$ meson decays
Source: arXiv:2609.02475 source file (2026-10-25)
Supplement: Supplementary file 1 [file appendix.tex]

% ===============================================================================
% Purpose: appendix to the standard template: standard symbol alises from Ulrik
% Author: Tomasz Skwarnicki
% Created on: 2009-09-24
% ===============================================================================

%{\noindent\normalfont\bfseries\Large Appendices}
\section*{Appendices}

\appendix
